# Supplementary material for: Lifting Weak Supervision To Structured Prediction
Source: arXiv:2211.13375 source file (2022-11-24)
Supplement: Supplementary file 1 [file fig_spaces.tex]

\begin{figure} 
\centering
 \begin{tikzpicture} [remember picture]
 
\node (rect) [rectangle, draw, minimum width=115mm, minimum height=85mm] at (0,0) {};
\node (rect2) [rectangle, draw, minimum width=100mm, minimum height=70mm] at (0,0) {};
\node (rect3) [rectangle, draw, minimum width=85mm, minimum height=55mm] at (0,0) {};
\node (rect4) [rectangle, draw, minimum width=70mm, minimum height=40mm] at (0,0) {};
\node (rect5) [rectangle, draw, minimum width=55mm, minimum height=25mm] at (0,0) {};
\node (rect6) [rectangle, draw, minimum width=40mm, minimum height=10mm] at (0,0) {};
\node[anchor=north] at (rect.north) {{Pseudo-metric Spaces [a), b)]}};
\node[anchor=north] at (rect2.north) {Semi-metric Spaces [a), b), c)]};
\node[anchor=north] at (rect3.north) {Metric Spaces [a), b),c), d)]};
\node[anchor=north] at (rect4.north) {Normed Vector Spaces};
\node[anchor=north] at (rect5.north) {Hilbert Spaces};
\node[] at (rect6.center) {Euclidean Spaces};
\end{tikzpicture}
\caption{Sub-spaces of pseudo-metric spaces}
\end{figure}
